# Supplementary material for: Effects of Interfaces on Human-Robot Trust: Specifying and Visualizing Physical Zones
Source: arXiv:2112.00779 source file (2021-12-01)
Supplement: Supplementary file 1 [file Supplement.pdf]

# Survey data

## Entry survey data

### Demographics

All questions had a “Prefer not to answer” option

1. What is your age? (5 yr brackets) - majority of participants were students

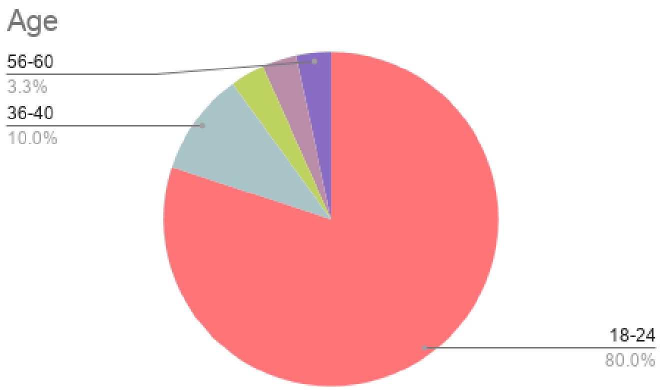


2. Gender (woman/man/non-binary)

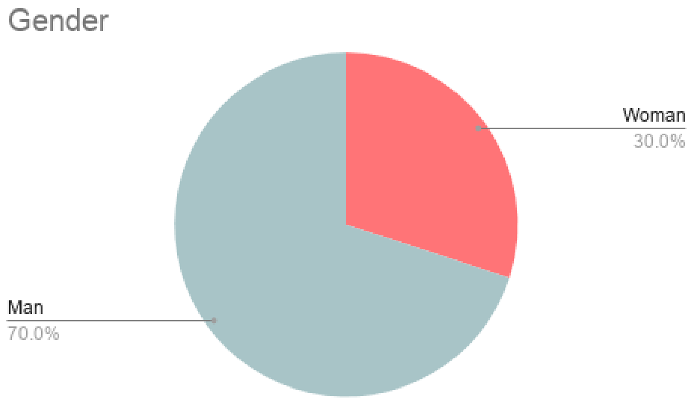


3. Education

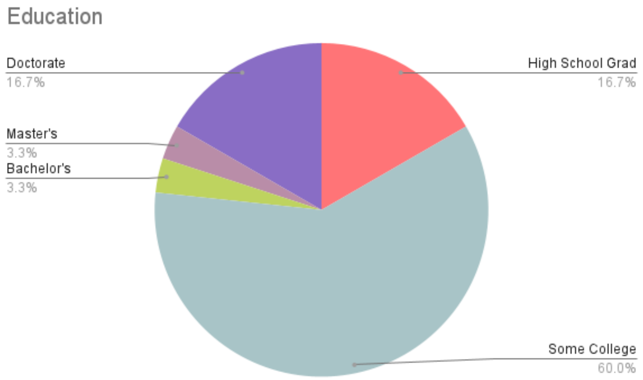


## Technology use

4. How many hours a day do you use technology for the following reasons? [2hr increments]

Q4 - How many hours a day do you use technology for the following reasons?

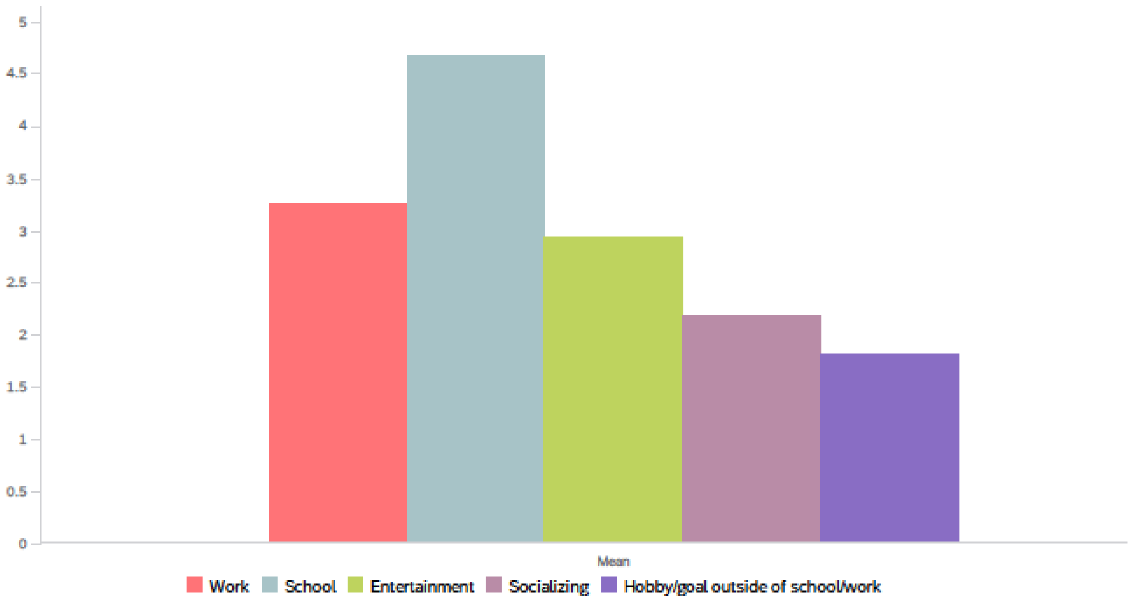


   a. Work, School, Entertainment, Socializing, Hobby/goal outside of school/work

5. How open are you to adopting new technology? Choose the option that best describes you.
   a. I want to be among the first people to try a new technology
   b. I will try a new technology after the first wave of people have tried it and given it positive reviews

c. I usually delay trying a new technology until I have to, or until it would be a bad business decision to keep resisting it

Q5 - How open are you to adopting new technology? Choose the option that best describes you.

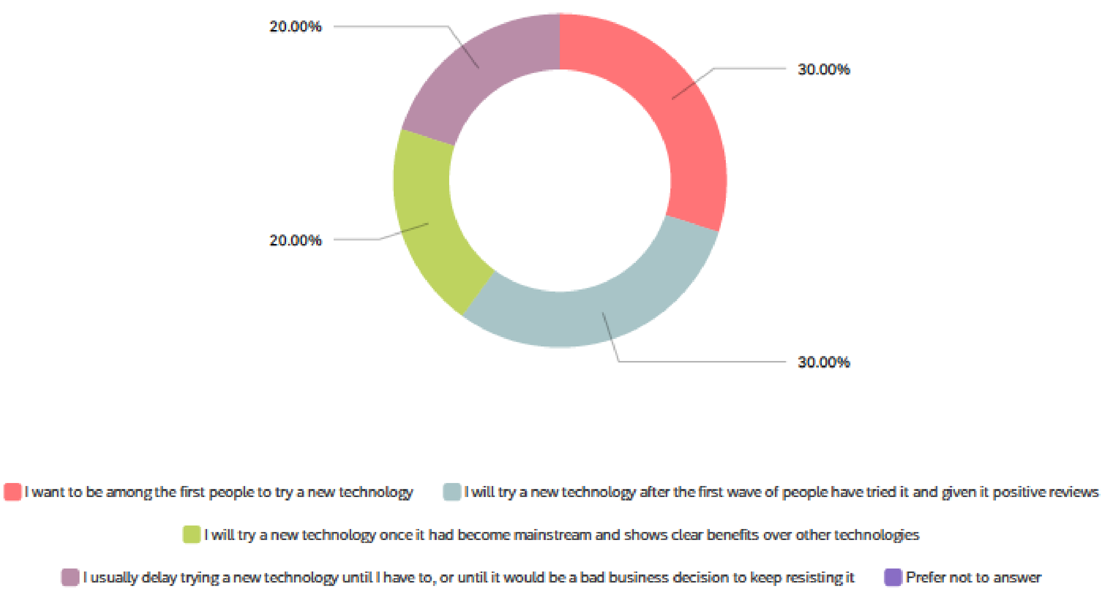

## Robot familiarity

6. What option best describes your familiarity with robots?
    a. I don't know what a robot is
    b. I have heard the term "robot" in conversation, but that's it
    c. I have only seen robots in TV and movies
    d. I have seen a video of a robot before
    e. I have personally been around a robot before
    f. I have driven remote-control devices (e.g., R/C cars/planes/helicopters, robotic toys)
    g. I have experience controlling or operating a robot
    h. I have experience building or programming a robot

Q6 - Which option best describes your familiarity with robots?

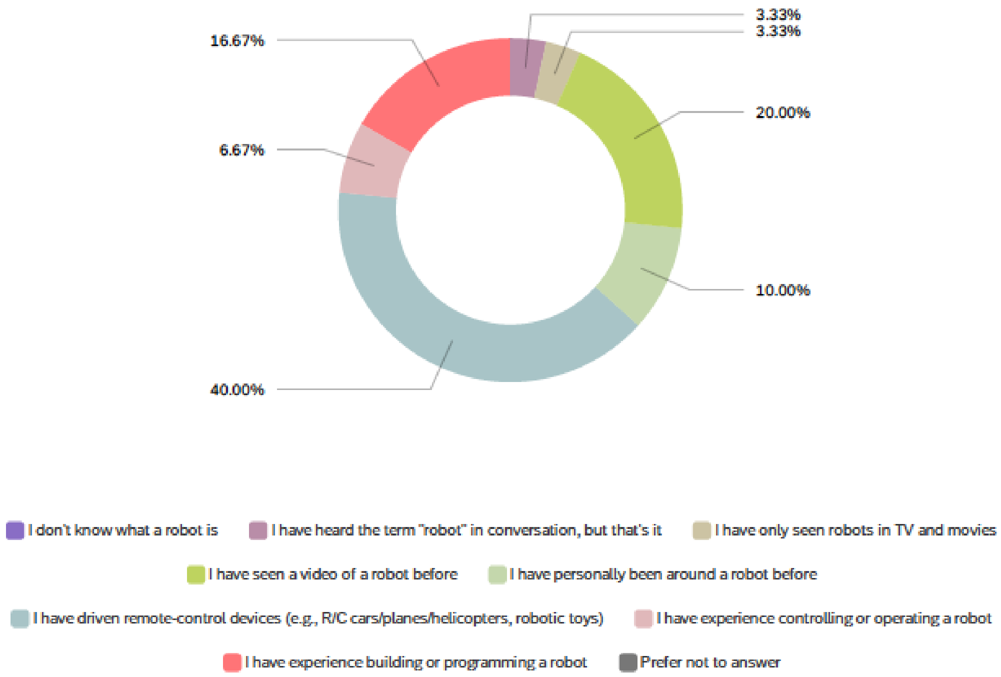


## NARS robot questions

7.

# Q8 - How much do you agree with the following statements?

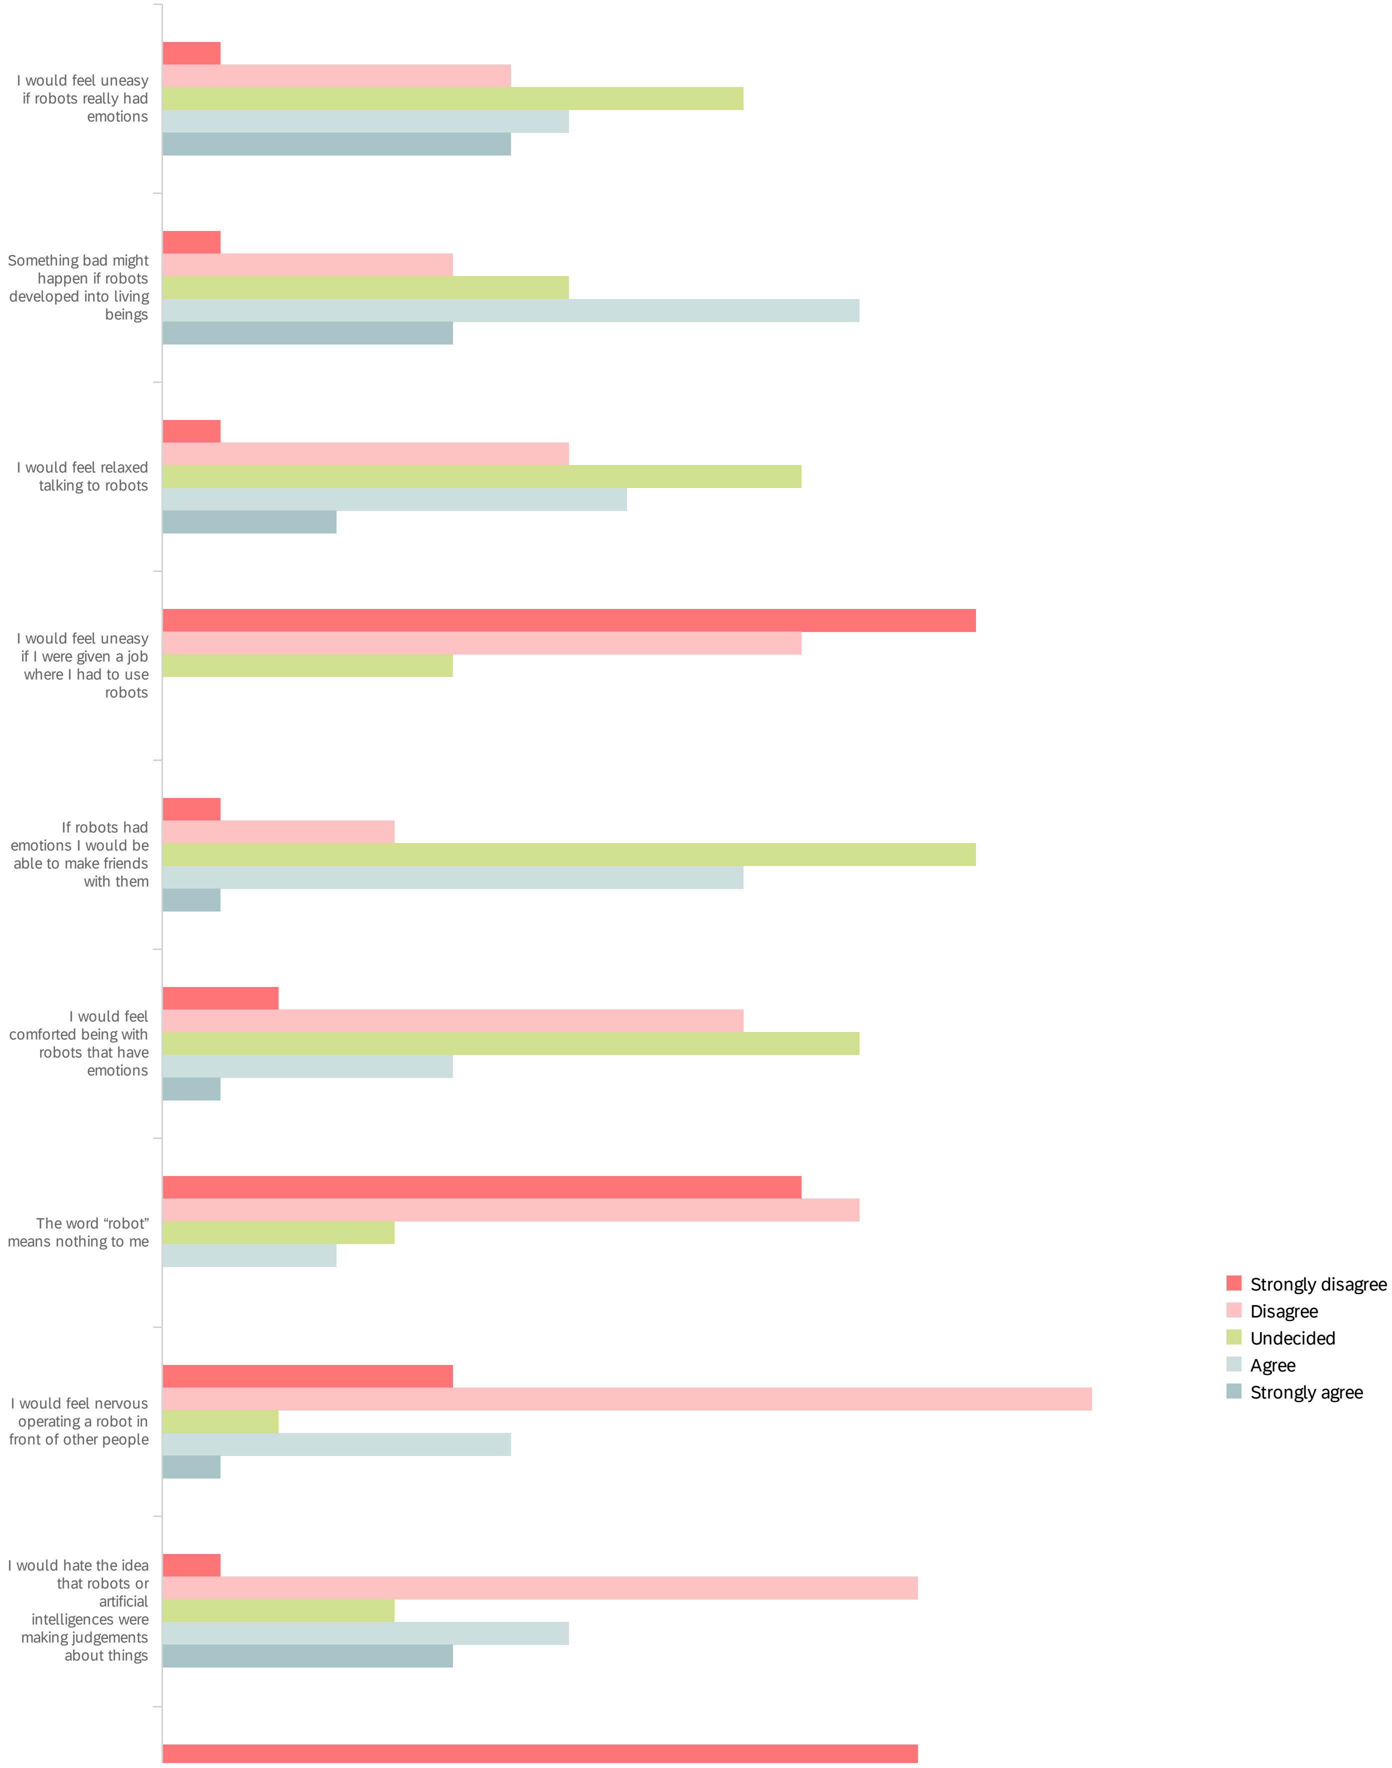

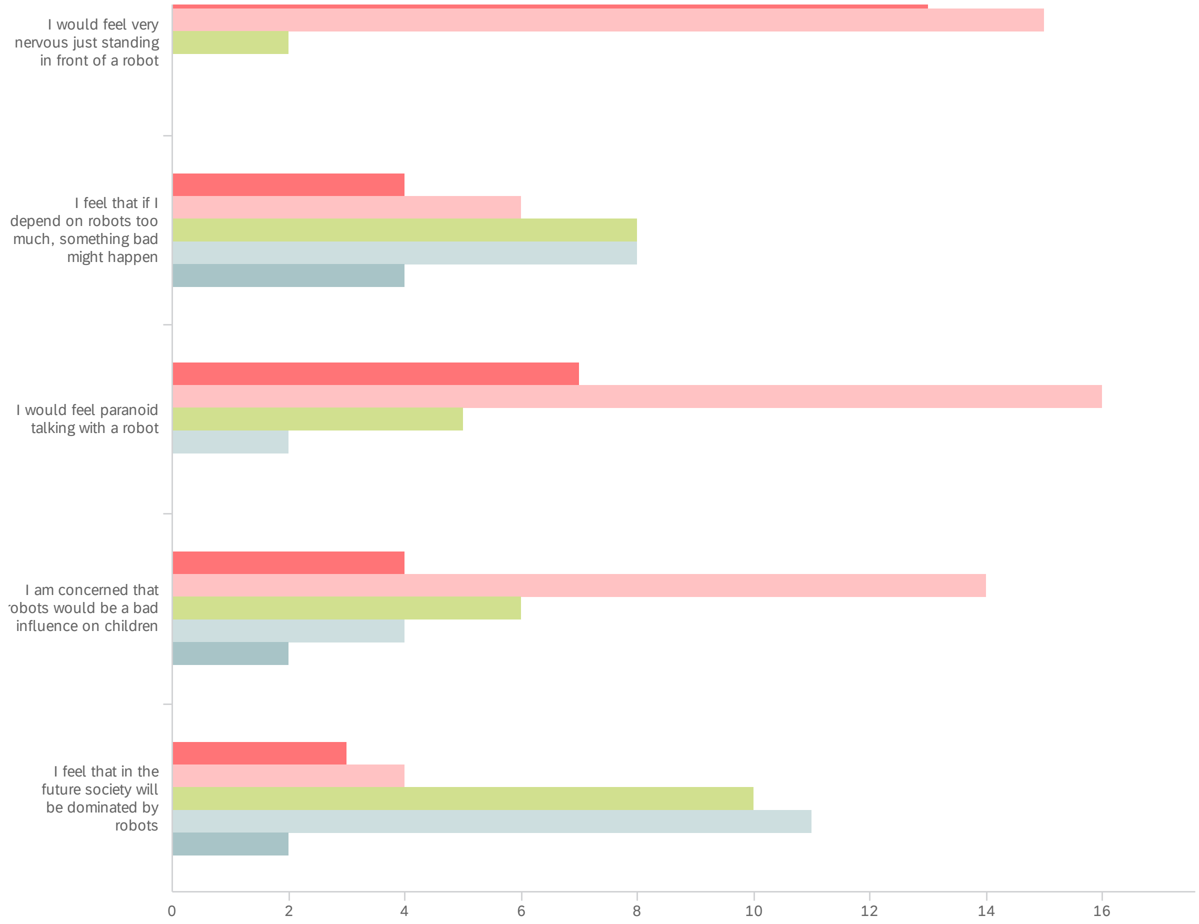
I would feel very nervous just standing in front of a robot
I feel that if I depend on robots too much, something bad might happen
I would feel paranoid talking with a robot
I am concerned that robots would be a bad influence on children
I feel that in the future society will be dominated by robots
0
2
4
6
8
10
12
14
16

## Self-efficacy, information gathering, tinkering questions

8. You won a robot vacuum cleaner in a raffle. Which approach best describes how you would set it up?
    a. Read the manual completely and then start setting it up
    b. Skim the manual until you find the setup instructions and then follow them step by step
    c. Start playing with the vacuum cleaner interface to see if you can set it up without reading the manual

Q9 - You won a robot vacuum cleaner in a raffle. Which approach best describes how you would set it up?

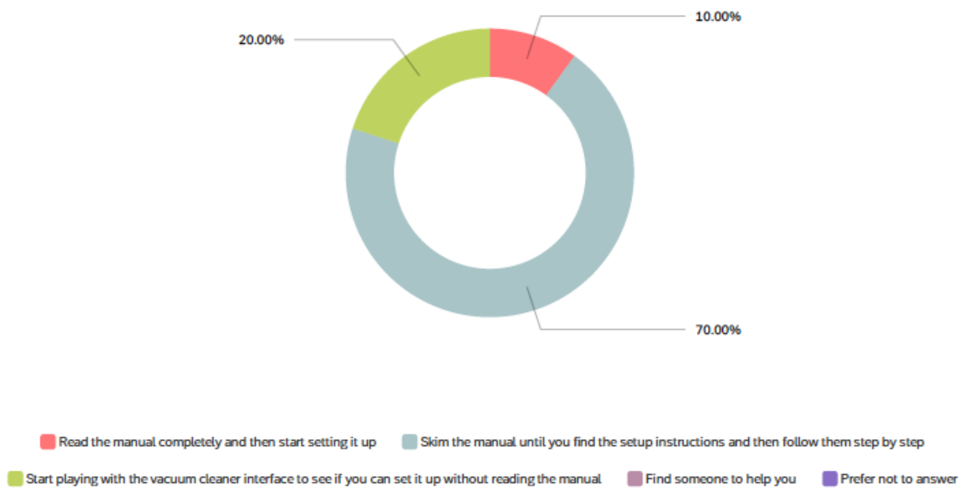


    d. Find someone to help you
9. If you get stuck setting up the robot vacuum cleaner, how likely is it that you would do any of the following things? (7 pt likert)
    a. Go online and look for a help video
    b. Go online and read advice
    c. Find a friend to set it up for you
    d. Call the company
    e. Send the robot vacuum cleaner back

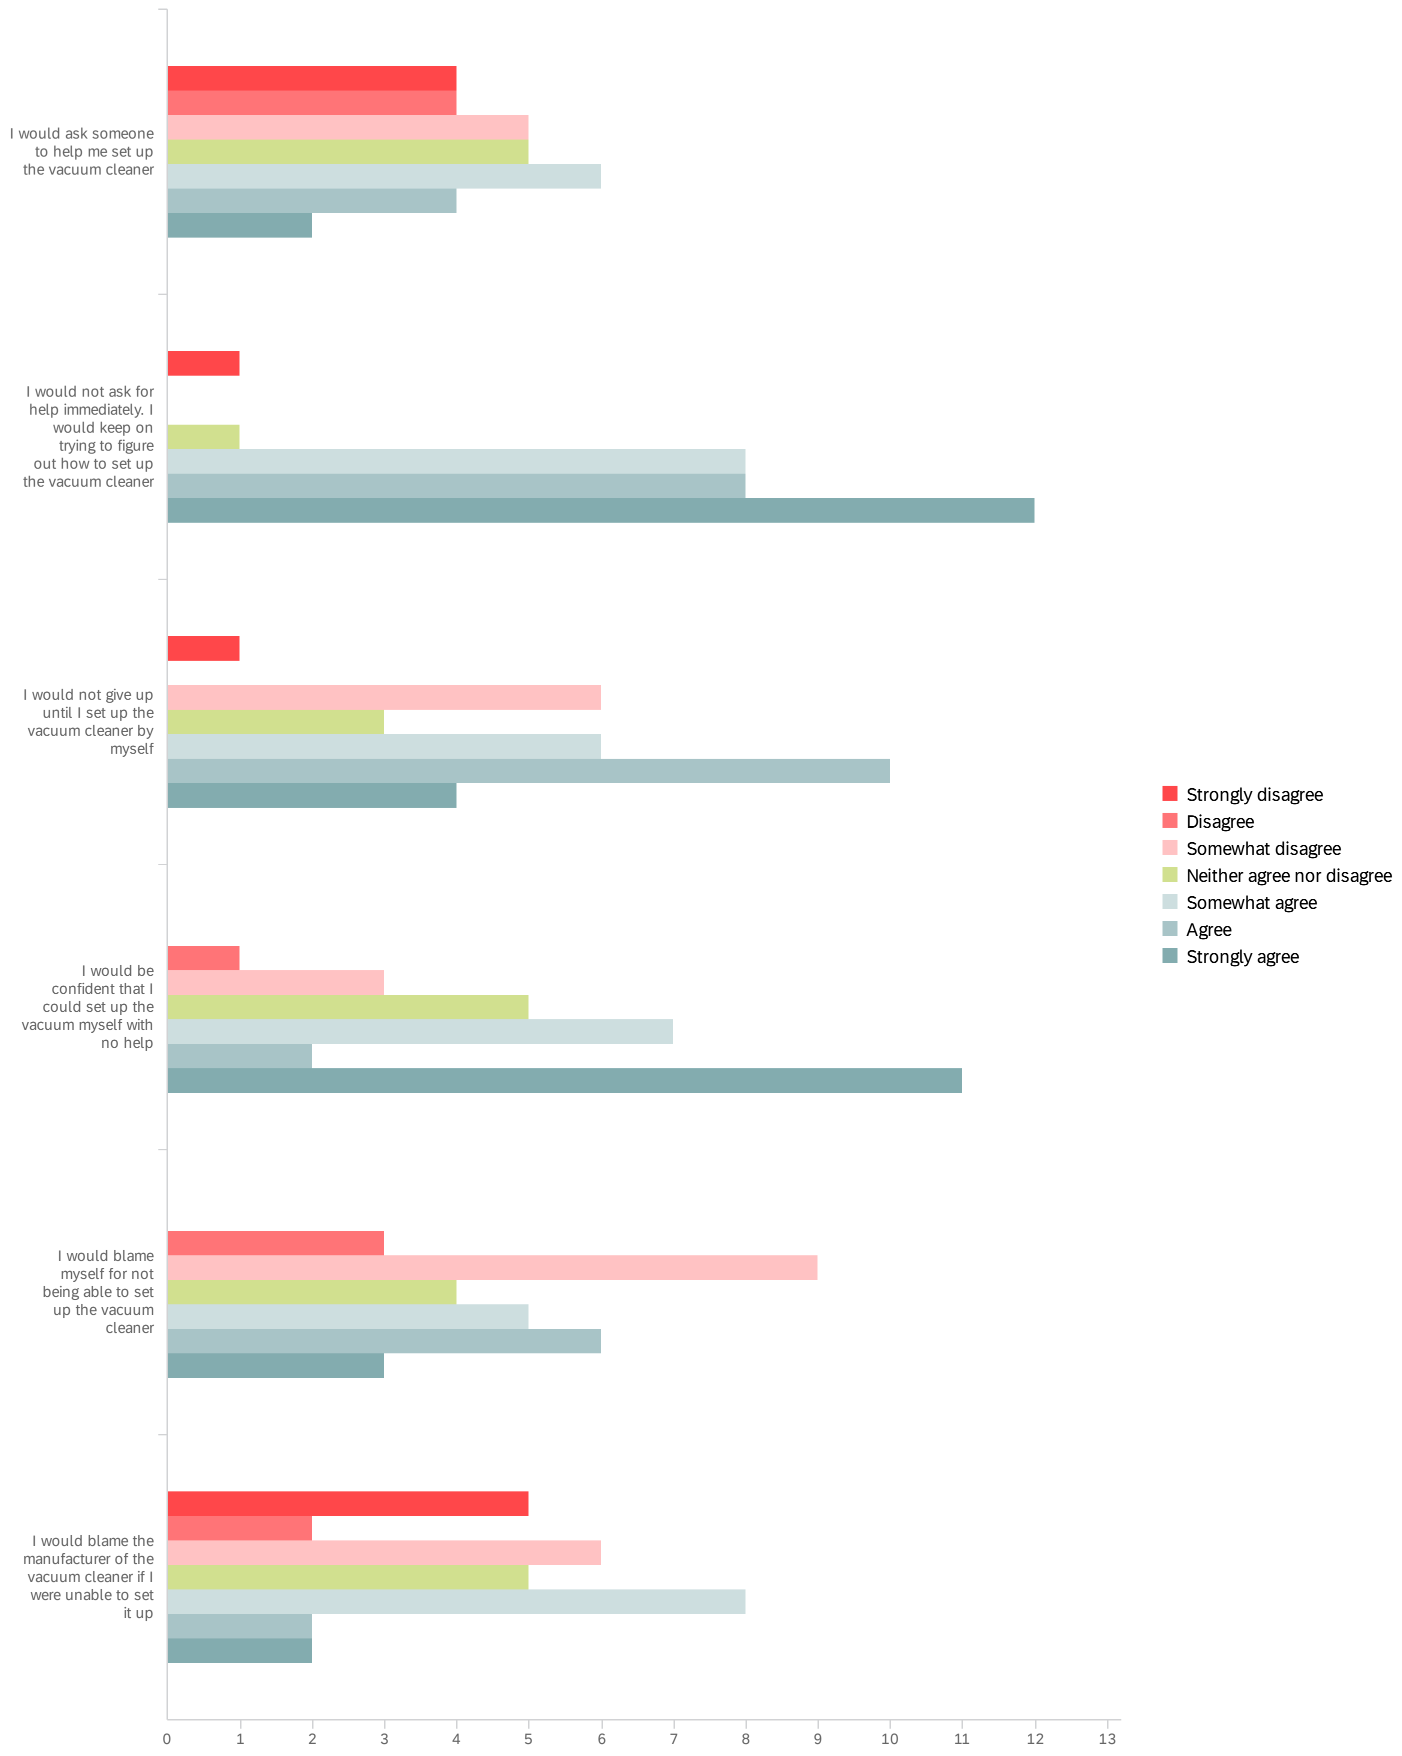

I would ask someone to help me set up the vacuum cleaner
I would not ask for help immediately. I would keep on trying to figure out how to set up the vacuum cleaner
I would not give up until I set up the vacuum cleaner by myself
I would be confident that I could set up the vacuum myself with no help
I would blame myself for not being able to set up the vacuum cleaner
I would blame the manufacturer of the vacuum cleaner if I were unable to set it up
0
1
2
3
4
5
6
7
8
9
10
11
12
13
Strongly disagree
Disagree
Somewhat disagree
Neither agree nor disagree
Somewhat agree
Agree
Strongly agree

10. How much do you agree with the following statements? (7 pt Likert)
    a. I would ask someone to help me set up the vacuum cleaner
    b. I would not ask for help immediately. I would keep on trying to figure out how to set up the vacuum cleaner
    c. I would not give up until I set up the vacuum cleaner by myself
    d. I would be confident that I could set up the vacuum myself with no help
    e. I would blame myself for not being able to set up the vacuum cleaner
    f. I would blame the manufacturer of the vacuum cleaner if I were unable to set it up

Q10 - If you get stuck setting up the robot vacuum cleaner, how likely is it that you would do any of the following things?

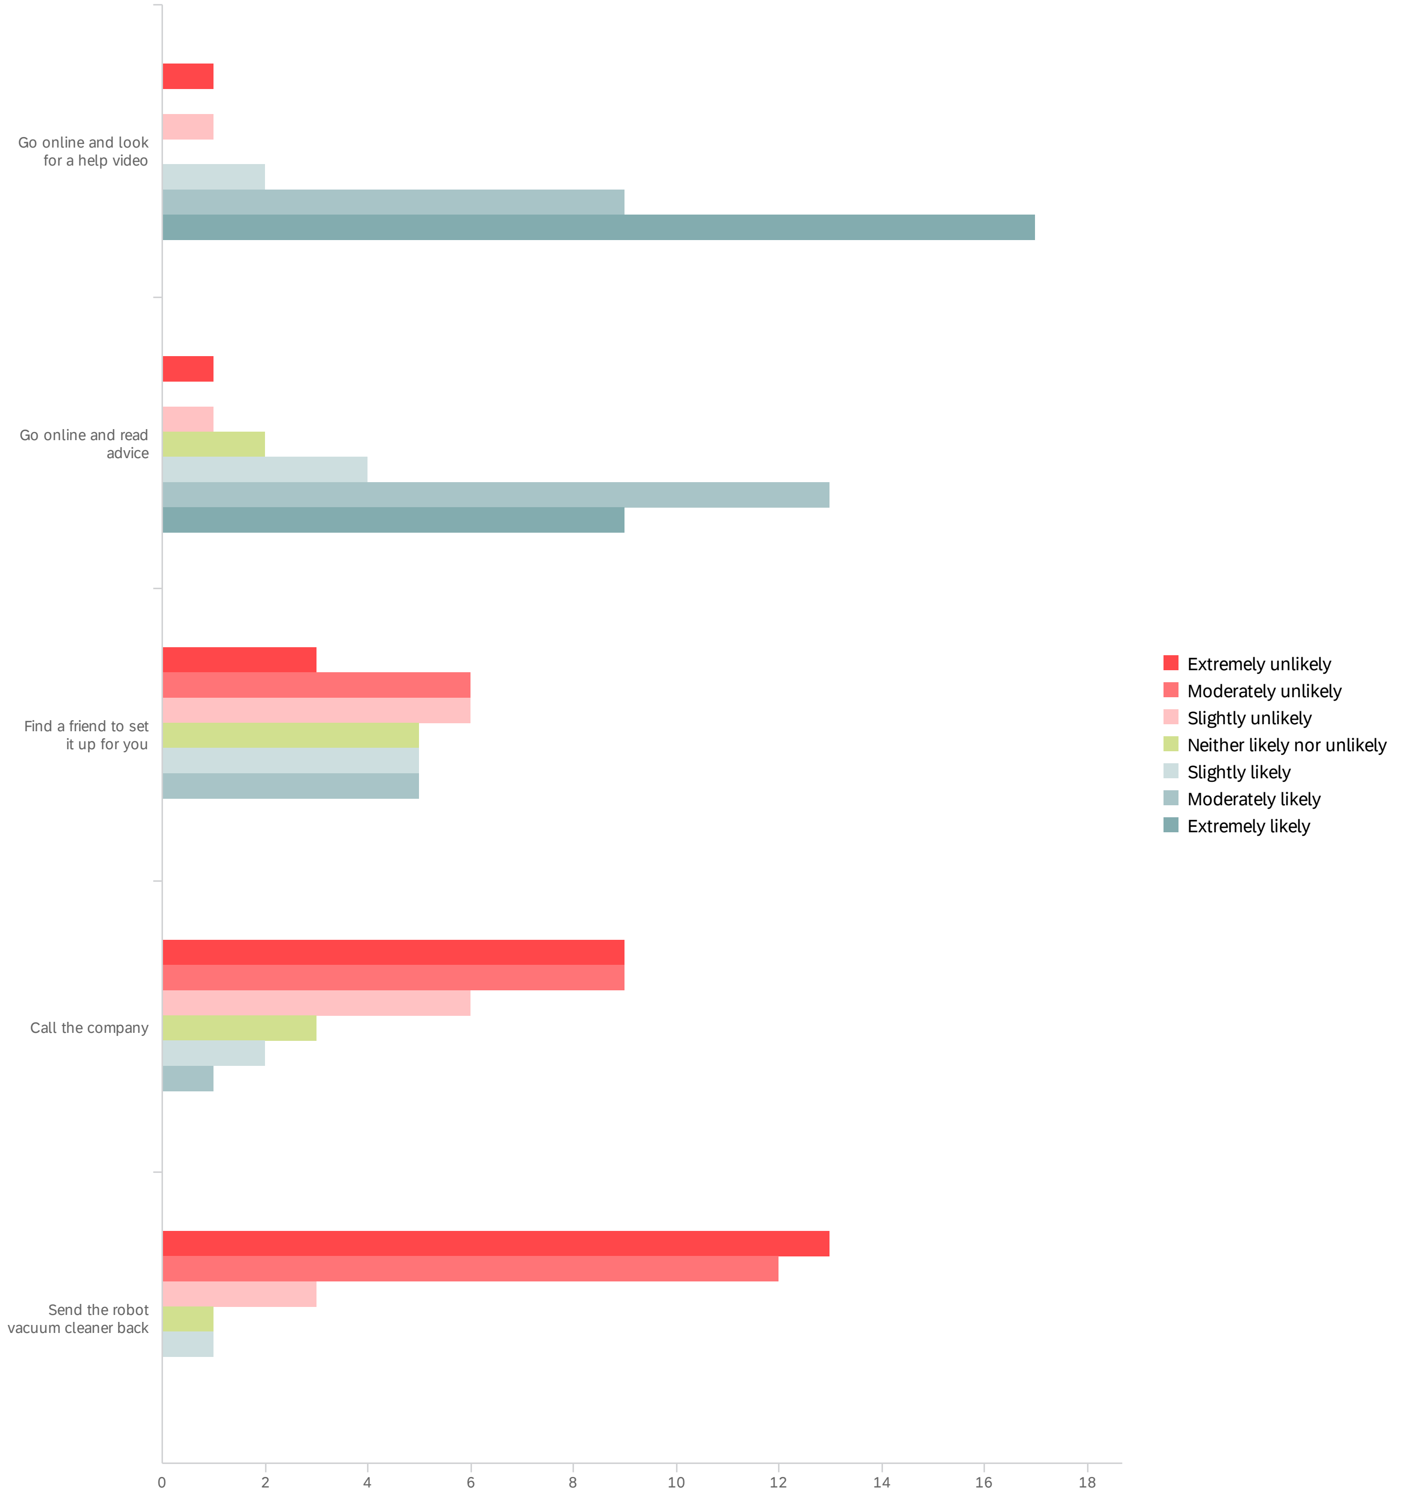

11. You successfully set up the robot vacuum cleaner and are ready to let it sweep. What would you do while the robot vacuumed for the first few times?
    a. I would let the vacuum cleaner move around on its own, but I would check up on it regularly
    b. I would set the vacuum cleaner to clean, and I would go do something else
    c. I would follow the vacuum cleaner around the first few times to make sure it was doing its job correctly

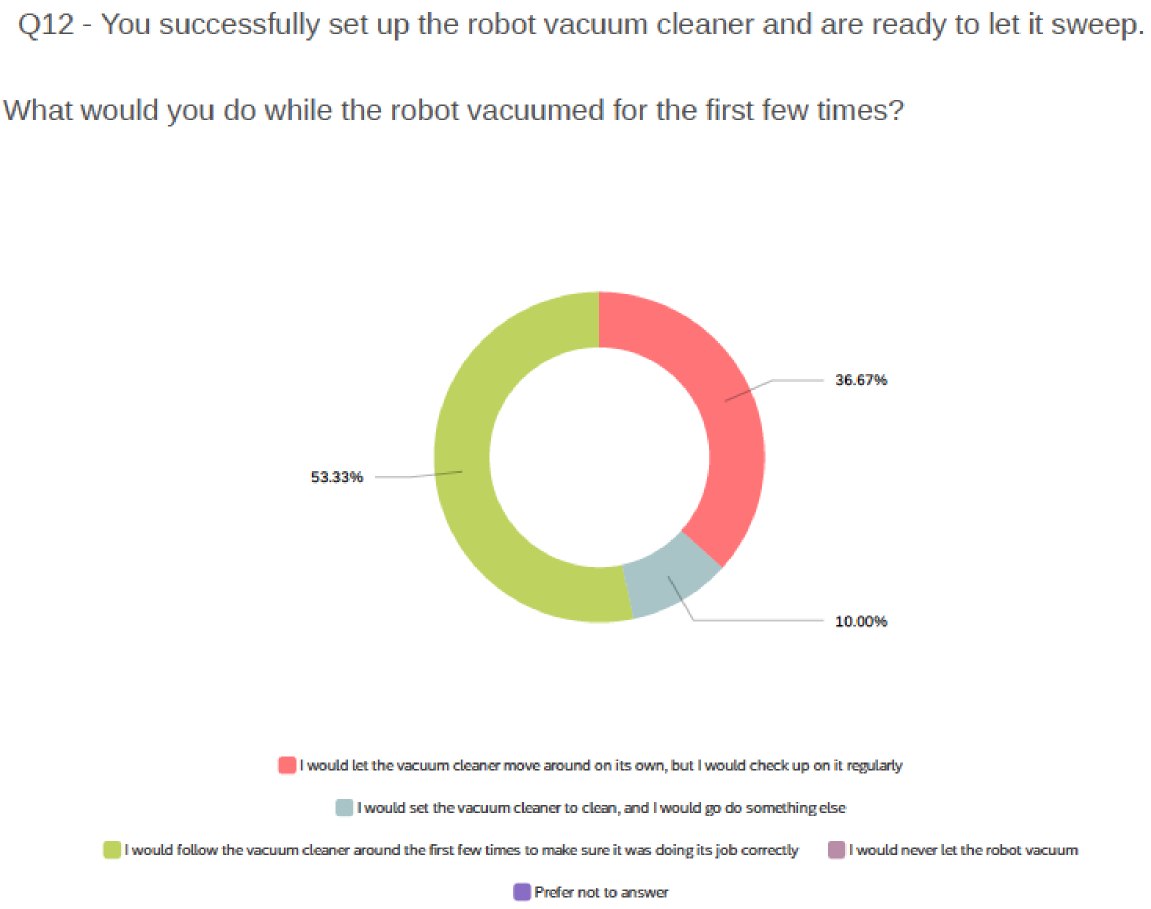


    d. I would never let the robot vacuum
12. How much would you trust the robot vacuum cleaner to do the following things the first few times it vacuumed? (7 pt likert)
    a. Not to break anything
    b. To clean properly without supervision
    c. To be near children or pets

Q13 - How much would you trust the robot vacuum cleaner to do the following things the first few times it vacuumed?

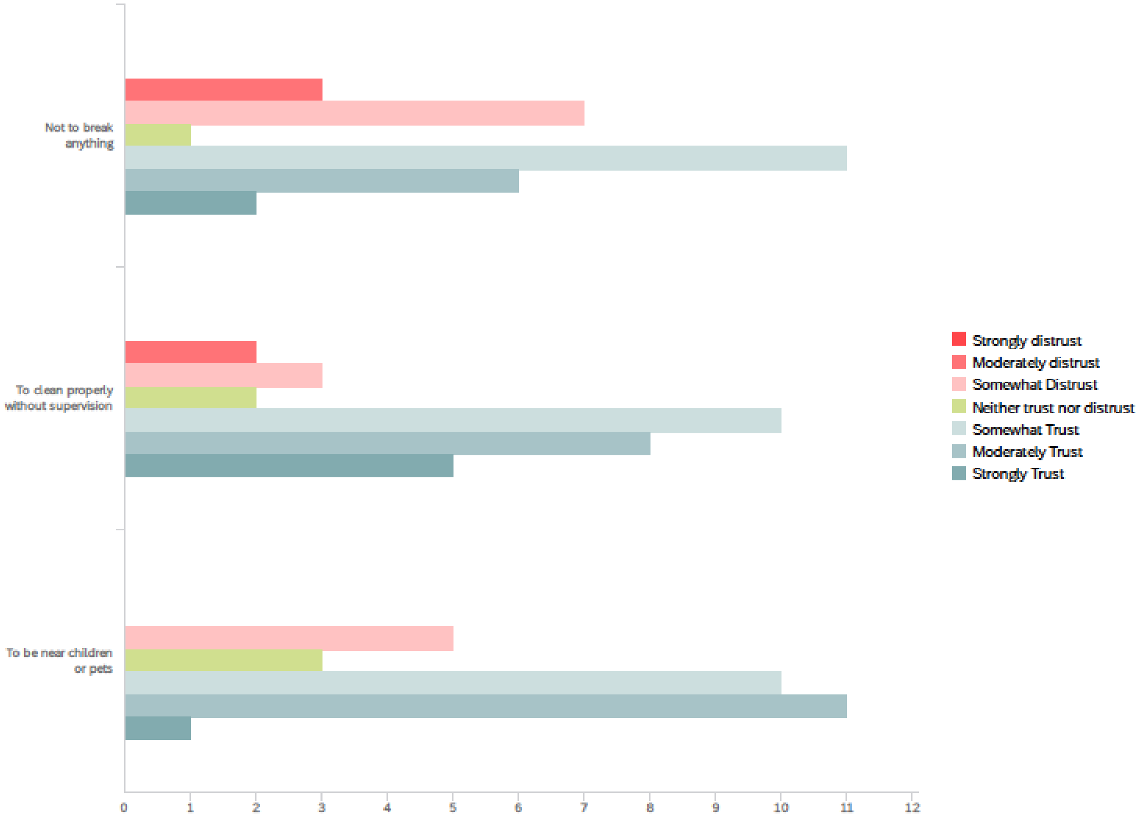


13. After the vacuum cleaner is set up, how would you feel about tinkering with settings to customize or explore the robot's features?
    a. I would spend so much time looking for new features that I may lose focus on what I set out to do originally
    b. I would look at a few specific features to make the vacuum cleaner work better, but I would not spend too much time on it
    c. I would not be interested in exploring new features, and I would change things only when I have to
    d. I would explore the features of the vacuum cleaners by reading step-by-step tutorials and videos rather than tinkering with its features
    e. I would be afraid of trying new settings because it may mess things up

Q14 - After the vacuum cleaner is set up, how would you feel about tinkering with settings to customize or explore the robot's features?

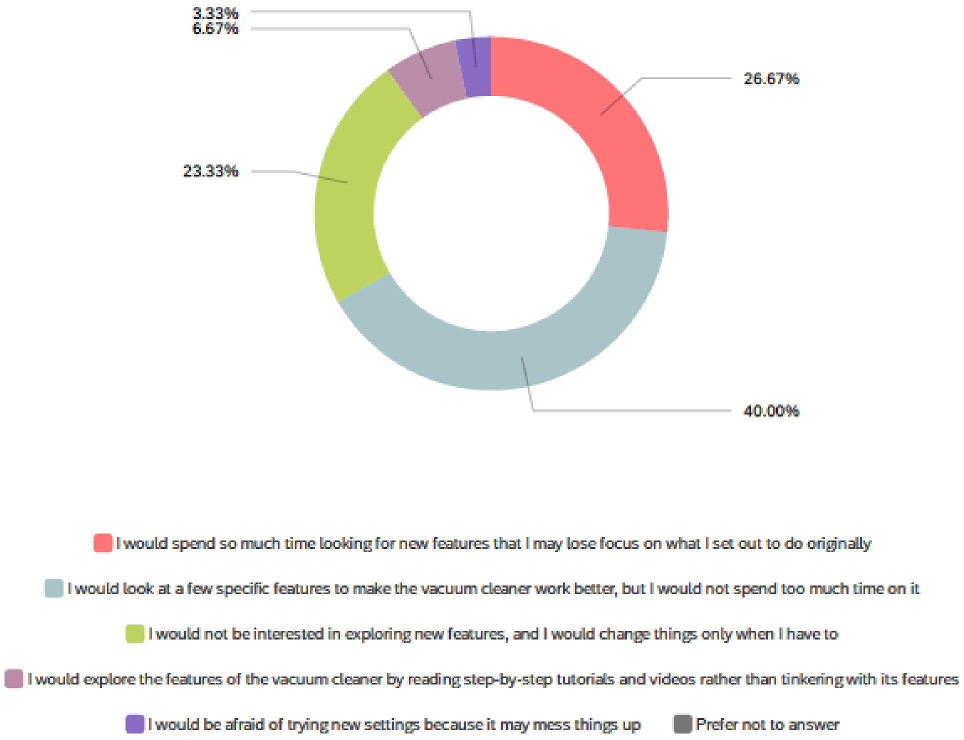

# Per task survey data

Three questions, recognize, able to avoid, actually avoid, followed by a question on feedback. The feedback question either asked if their answer would have changed if they had seen or NOT seen the feedback

General trends:

- Decrease in trust remember -> able to avoid -> actually avoid
- AR/Physical - feedback increases trust
- Map - feedback decreases trust

## Survey specifics: Trust

Question wording: How often do you think the robot do the following things? (7-pt likert scale, Never->Always)

1. Be able to recognize where it should go
2. Be able to avoid where it should not go
3. Actually avoid where it should not go

Answers to survey questions (as Likert scale) in recognize -> able to avoid -> actually avoid order

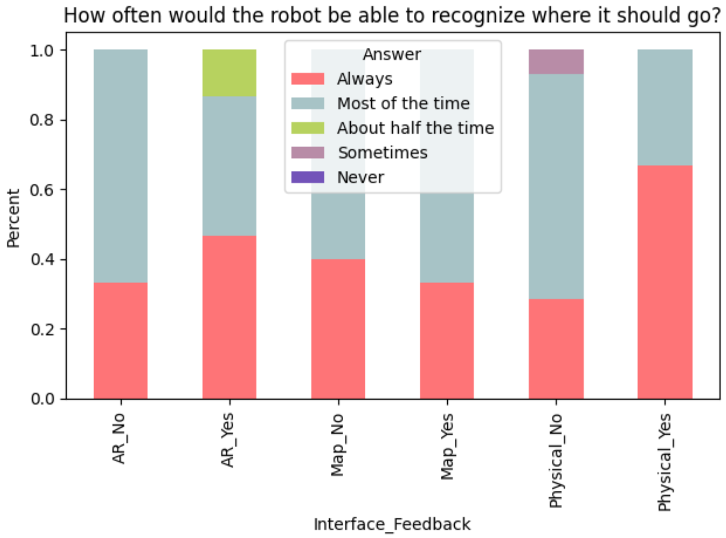

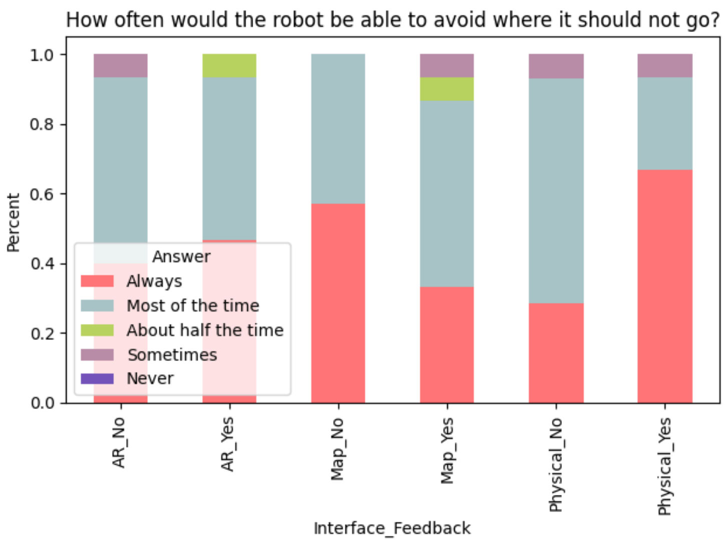


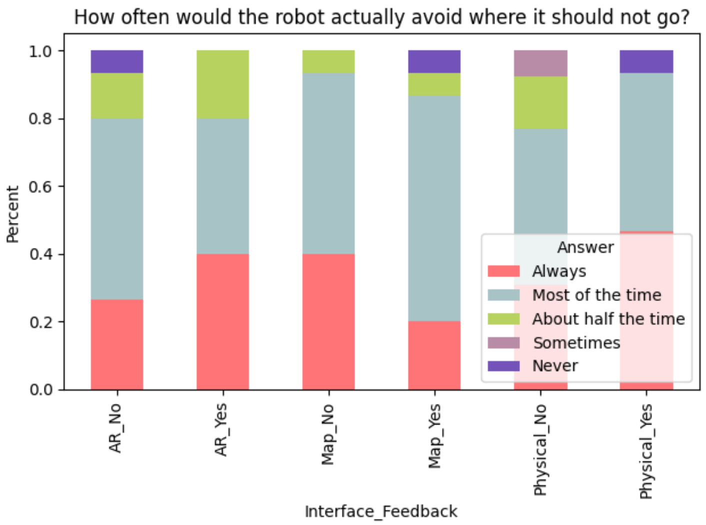


Likert scale converted to 1-5 scale
Green: Feedback increased trust
Yellow: Feedback neither increased nor decreased trust
Red: Feedback decreased trust

| Interface/Feedback combo | | | | | | | | |
|---|---|---|---|---|---|---|---|---|
| | | Never | Sometimes | Half the time | Most of the time | Always | | |
| recognize | Physical/Physical | 0 | 0 | 0 | 0.333333 | 0.666667 | | 4.666667 |
| | Physical/None | 0 | 0.071429 | 0 | 0.642857 | 0.285714 | | 4.142856 |

| | | | | | | | | |
|---|---|---|---|---|---|---|---|---|
| | Map/Map | 0 | 0 | 0 | 0.666667 | 0.333333 | | 4.333333 |
| | Map/None | 0 | 0 | 0 | 0.6 | 0.4 | | 4.4 |
| | AR/AR | 0 | 0 | 0.133333 | 0.4 | 0.466667 | | 4.333334 |
| | AR/None | 0 | 0 | 0 | 0.666667 | 0.333333 | | 4.333333 |
| | | | | | | | | |
| avoid | Physical/Physical | 0 | 0.066667 | 0 | 0.266667 | 0.666667 | | 4.533337 |
| | Physical/None | 0 | 0.076923 | 0 | 0.642857 | 0.285714 | | 4.153844 |
| | Map/Map | 0 | 0.066667 | 0.066667 | 0.533333 | 0.333333 | | 4.133332 |
| | Map/None | 0 | 0 | 0 | 0.428571 | 0.571429 | | 4.571429 |
| | AR/AR | 0 | 0 | 0.066667 | 0.466667 | 0.466667 | | 4.400004 |
| | AR/None | 0 | 0.066667 | 0 | 0.533333 | 0.4 | | 4.266666 |
| | | | | | | | | |
| actually avoid | Physical/Physical | 0.066667 | 0 | 0 | 0.466667 | 0.466667 | | 4.26667 |
| | Physical/None | 0 | 0.076923 | 0.153846 | 0.461538 | 0.307692 | | 3.999996 |
| | Map/Map | 0.066667 | 0 | 0.066667 | 0.666667 | 0.2 | | 3.933336 |
| | Map/None | 0 | 0 | 0.066667 | 0.533333 | 0.4 | | 4.333333 |
| | AR/AR | 0 | 0 | 0.2 | 0.4 | 0.4 | | 4.2 |
| | AR/None | 0.066667 | 0 | 0.133333 | 0.533333 | 0.266667 | | 3.933333 |

## Survey specifics: Feedback

Question if they **saw** the feedback:

- [Physical] If you had not seen the robot drive around the no-go region, how much would your answers to the previous question have changed?
- [AR] If you had not seen the virtual fence surrounding the no-go region, how much would your answers to the previous question have changed?
- [Map] If you had not seen the no-go region shaded red on the map, how much would your answers to the previous question have changed?

Question if they **did not see** the feedback: if you had seen [etc]

Answers were the same 3-pt likert in either case:

- A great deal
- A lot
- A moderate amount

- A little
- None at all

AR_No means they saw the AR interface but with no feedback, AR_Yes means they saw they saw the AR interface with the virtual fence

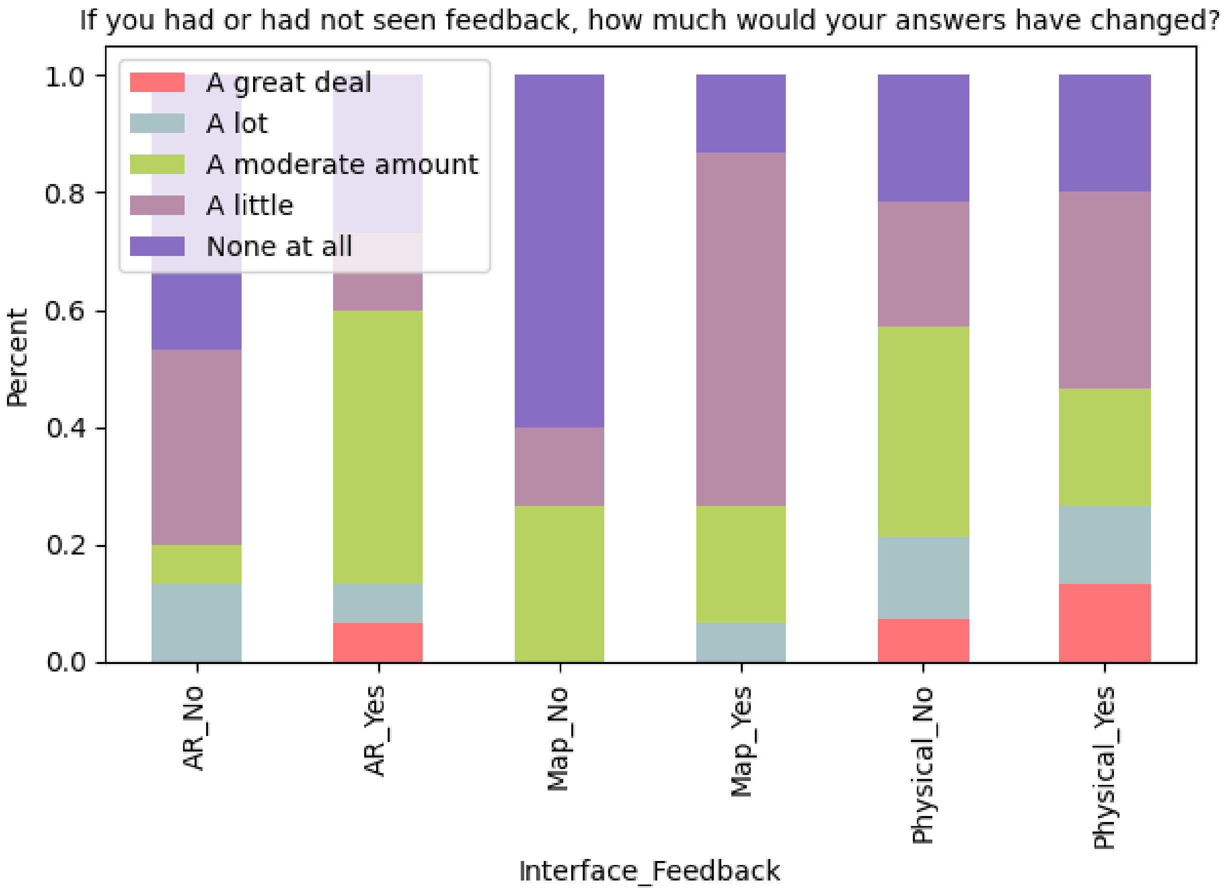


| Q7,8,9,10,11: If you had/had not seen feedback, how much would your answers have changed? | | | | | | Average |
|---|---|---|---|---|---|---|
| | None at all | A little | A moderate amount | A lot | A great deal | |
| Physical/Physical | 0.2 | 0.333333 | 0.2 | 0.133333 | 0.133333 | 2.666663 |
| Physical/None | 0.214286 | 0.214286 | 0.357143 | 0.142857 | 0.071429 | 2.64286 |

| | | | | | | |
|---|---|---|---|---|---|---|
| Map/Map | 0.133333 | 0.6 | 0.2 | 0.066667 | 0 | 2.200001 |
| Map/None | 0.6 | 0.133333 | 0.266667 | 0 | 0 | 1.666667 |
| AR/AR | 0.266667 | 0.133333 | 0.466667 | 0.066667 | 0.066667 | 2.533337 |
| AR/None | 0.466667 | 0.333333 | 0.066667 | 0.133333 | 0 | 1.866666 |

# Exit survey data

This survey was given after the last task. It measured usefulness and ease of use for each interface. It also measured overall competency of the robot.

## Usefulness/easy to use

How useful did you find each interface for creating a no-go region? (7-pt Likert from Extremely useless to Extremely useful)

Ease of use: How easy did you think each interface was to use? (7-pt Likert from Extremely difficult to Extremely easy)

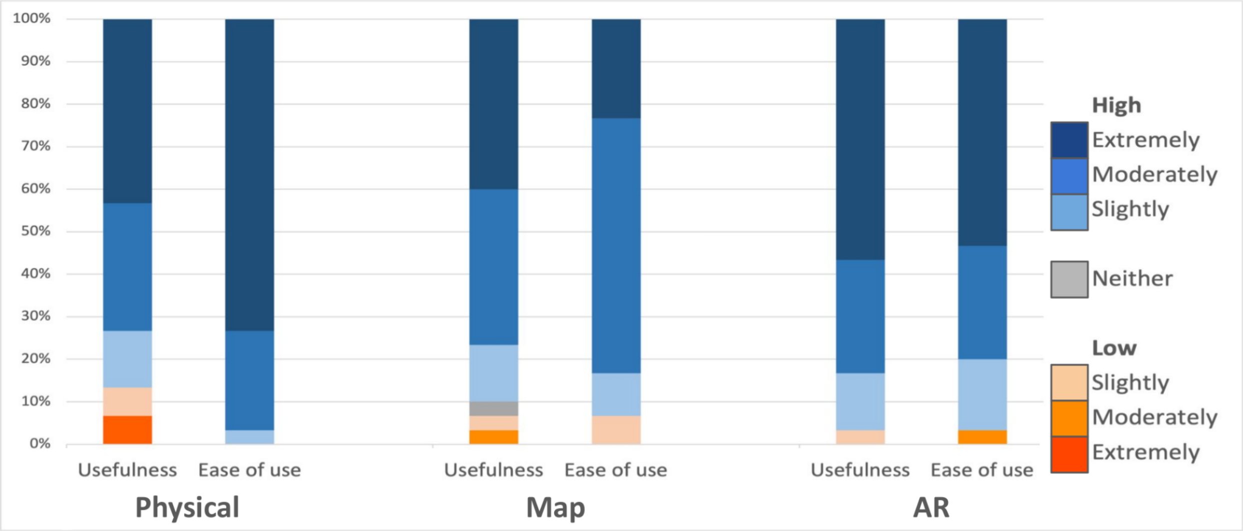


| | | | | | | | | |
|---|---|---|---|---|---|---|---|---|
| Q12: Usefulness of each Interface | | | | | | | | |

| | Extremely useless | Moderately useless | Slightly useless | Neither | Slightly useful | Moderately useful | Extremely useful | Average useful |
|---|---|---|---|---|---|---|---|---|
| Physical | 0.066667 | 0 | 0.066667 | 0 | 0.133333 | 0.3 | 0.433333 | 0.933333 |
| Map | 0 | 0.033333 | 0.033333 | 0.033333 | 0.133333 | 0.366667 | 0.4 | 0.966662 |
| AR | 0 | 0 | 0.033333 | 0 | 0.133333 | 0.266667 | 0.566667 | 0.766664 |
| | | | | | | | | |
| Q18: Ease of Use of each Interface | | | | | | | | |
| | Extremely difficult | Moderately difficult | Slightly difficult | Neither | Slightly easy | Moderately easy | Extremely easy | Average easy |
| Physical | 0 | 0 | 0 | 0 | 0.033333 | 0.233333 | 0.733333 | 0.166665 |
| Map | 0 | 0 | 0.066667 | 0 | 0.1 | 0.6 | 0.233333 | 0.700001 |
| AR | 0 | 0.033333 | 0 | 0 | 0.166667 | 0.266667 | 0.533333 | 0.900001 |

## Robot skills

General trend: People perceived the robot as moderately competent, largely capable of avoid the no-go region, but in practice may not.

How competent do you think the robot is? (7-pt Likert from Not competent to Extremely competent)

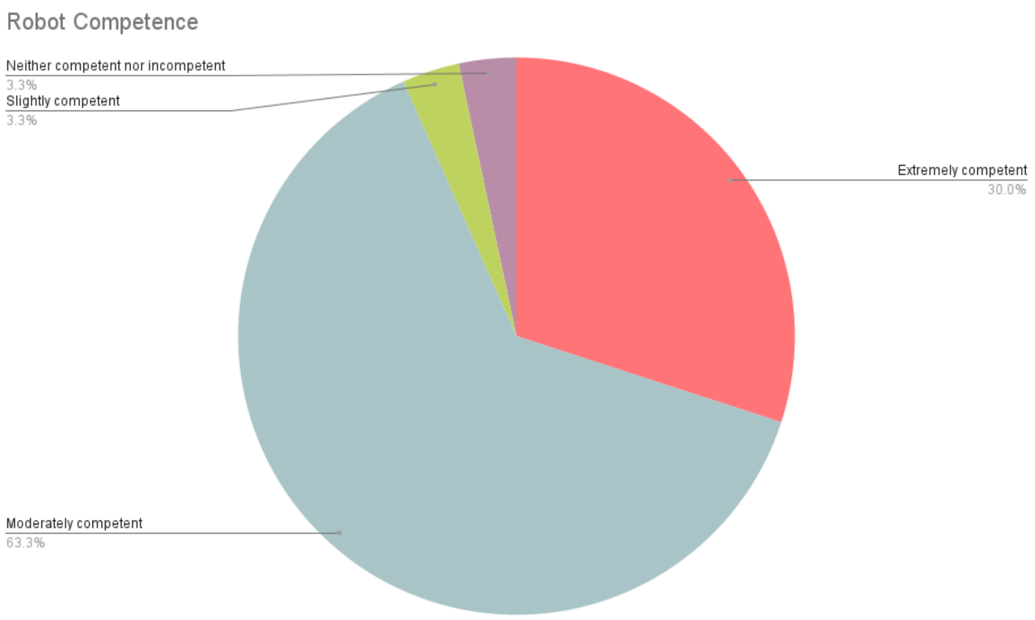


Do you think the robot is capable of avoiding the no-go region? (7-pt Likert from Definitely no to Definitely yes)

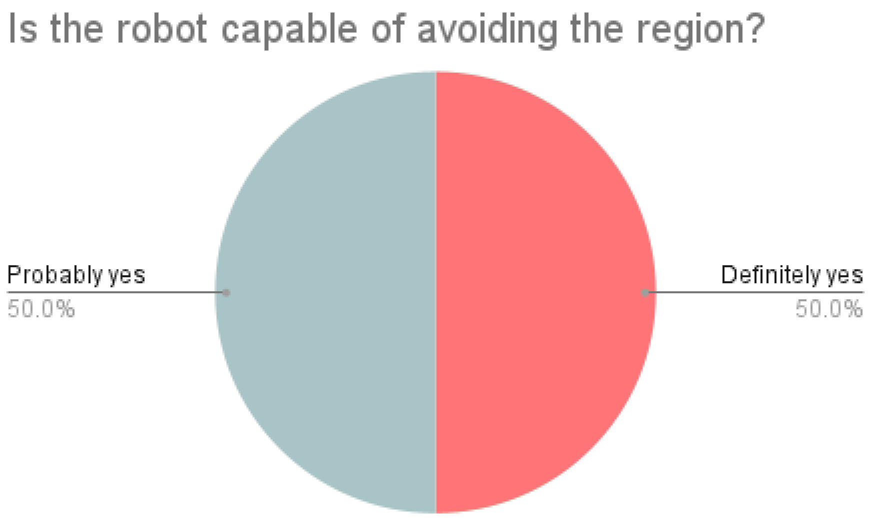


Do you think the robot would choose to enter a region it was told not to go into, even if it was capable of avoiding the region? (7-pt Likert from Definitely not to Definitely yes)

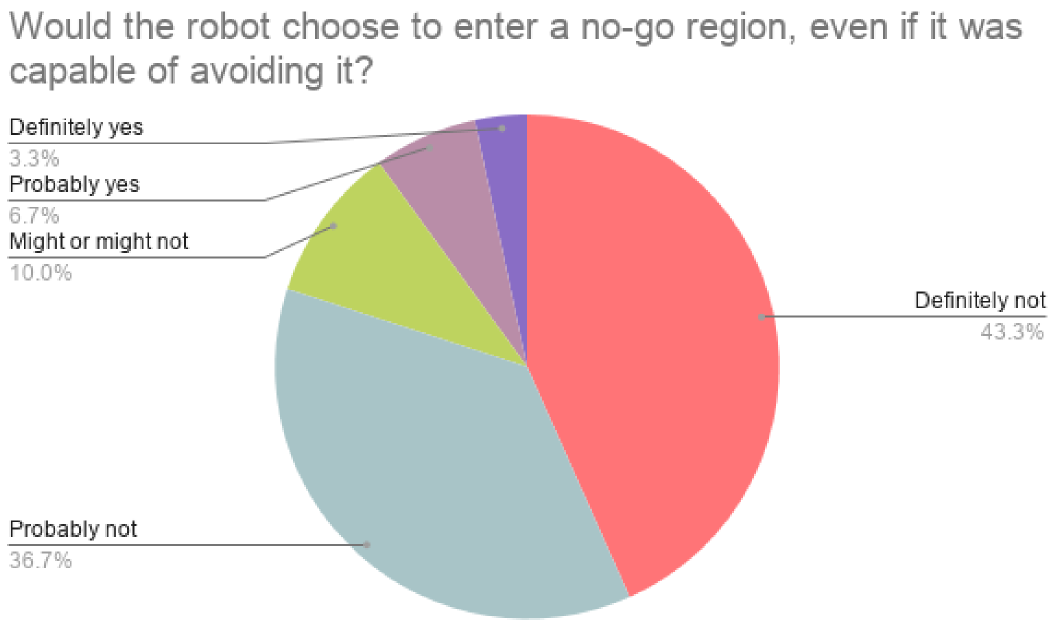


Open-ended text question: Of the things you have seen during the study, what made you trust that the robot would avoid the no-go region the most?

Summary: Most of these are some version of “I saw feedback”, with the robot driving around being the most common, and the fence/virtual cones being the second. Unusual responses are highlighted in green. Interestingly, only one person said “because I set the cones”

- because it did avoid it
- Seeing the robot actually move. It definitely gave itself a lot of space around where I gave it a no-go zone. I put the cones right next to the table legs and it move like a half a foot away from the zone, getting no where near the borders.
- The video of the robot avoiding the no-go region.
- AR Map with the virtual fence, where the user can see where the no-go region is
- the video of the robot avoiding the area
- Running the first test where it went around the no go region
- The video demonstration
- Seeing the map that it has of the room made increased my trust in it avoiding the no-go region. Compared to the cones and the AR fence, the map better demonstrates what the robot actually knows/does.
- The no-go region that has been set into the robot virtually and electronically would adjust its movement
- Seeing it actually avoid the no-go region. Also the cones made me trust the robot a little more.
- The AR interface seemed like the most reassuring method, seeing in 3D the area fenced off would be reassuring to a customer with potentially expensive items in that area. The map

interface seemed least effective as there could be user error and the physical interface is a decent method.

- The physical placing of the cones, followed by the mapping software.
- Visually seeing the robot avoid the no-go region.
- the video of it moving around the no-go region
- Allowing me to create the no-go region.
- The way it made sure to turn at the corners of the no-go region showed its adherence to ensuring it does not violate its command
- The map interface
- Because it demonstrated that it can do that through the cone test.
- Well it's not sentient as far as I'm aware, so it shouldn't be entering any regions it's not supposed to. Plus I watched it avoid the region once, so I know it CAN avoid the region
- [someone] implemented the no-go robot behavior
- Thej Augmented reality interface, because it most effectively bridges the virtual and physical world and gives you confirmation that the boundaries exist exactly where you meant them to be, whereas the physical interface does not inspire confidence that the robot actually recognizes where the boundaries are.
- Past experience with robots
- the virtual cones in the ar interface
- When there was a technology-based component to mapping out the no-go region/when I got see to the robot avoid the no-go region
- the administrator
- human determined parameters for what is "go" vs. "no-go"
- the inclusion of AR markers allow for the most flexibility
- AR interface
- The physical demonstration of the robot moving around the no go region

What else that you haven't seen would increase your trust that the robot would avoid the no-go region?

- Give them a name! Other than that, I do trust pretty much as much as I can.
- seeing it avoid it multiple times
- The robot moving and avoiding the no-go region in person.
- seeing it avoid the area in real life
- Maybe seeing the path of the robot in the app before it actually goes to the region it's supposed to
- I think seeing the camera/sensor data from the robot would, to some extent, increase my trust in the robot to avoid the no-go region. Like the map, this is more reflective of what the robot senses and could increase trust in its ability to know where to go and not go.
- Its long-term memory (if applicable) from the previous settings
- Seeing it go around the perimeter of the no-go region to prove it knows where it is.
- The effectiveness of the robot in real life, right now it has all been either hypothetical or in video so I would like to see it in person.
- Having the robot "see" the duct tape on the ground for other tests and use it as a no go area.

- Seeing the robot avoid the no-go region multiple times would increase my trust.
- the design behind the robot, like it's sensors wheels
- Seeing the robot move around and avoid the no-go region.
- Making the no-go region more like a maze and seeing whether the robot could \ navigate a tricky path would be further proof that it could avoid the no-go region
- Confirmation from the robot itself
- The robot seems like it was poorly designed so maybe working on the hardware. People tend to trust something that looks more professional.
- If I had gotten to see the robot avoid the no-go region for all of the different interfaces, I would feel a lot better. The AR cones didn't look very set in stone. Depending on the angle I held the camera at, they were in different locations.
- robots should err on the side of caution
- A demonstration of the robot avoiding the region automatically even when it is steered toward the area manually by a driver.
- Trust in the general ability of people creating the robot
- a physical fence
- I'm not sure
- My own robot vacuum.
- programming that depends on input for "go" vs. "no-go"
- highlighted proximity of robot intent
- have the no-go region appear on the robot's computer display
- More physical demonstrations of the robot avoiding no go regions, for the other types of interfaces too
